# Supplementary material for: Observation of a Modulational Instability in Bose-Einstein condensates
Source: arXiv:1703.07502 source file (2017-10-09)
Supplement: Supplementary file 1 [file observation-modulational-instability-supp.pdf]

# Observation of modulational instability in Bose-Einstein condensates: Supplemental Material

P.J. Everitt[1], M.A. Sooriyabandara[1], M. Guasoni[2], P.B. Wigley[1], C.H. Wei[1,3], G.D. McDonald[1], K.S. Hardman[1], P. Manju[1], J.D. Close[1], C.C.N. Kuhn[1], S.S. Szigeti[4], Y.S. Kivshar[2], and N.P. Robins[1]
[1]*Department of Quantum Science, Research School of Physics and Engineering, Australian National University, Canberra ACT 2601, Australia*
[2]*Nonlinear Physics Center, Research School of Physics and Engineering, Australian National University, Canberra ACT 2601, Australia*
[3]*Department of Instrument Science and Technology, College of Mechatronic Engineering and Automation, National University of Defense Technology, Changsha 410073, China*
[4]*Department of Physics, Centre for Quantum Science, and Dodd-Walls Centre for Photonic and Quantum Technologies, University of Otago, Dunedin 9010, New Zealand*

## I. SOLITON ENUMERATION

The number of solitons formed after each experimental run was quantified using an image processing algorithm (Fig. [S1]). The images are firstly de-noised with a discrete cosine transform (DCT) threshold filter. A binary threshold (60% of peak image intensity) is then applied. The number of resulting solitons is then found by counting the morphological components.

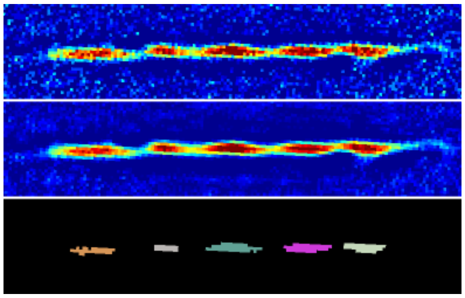

FIG. [S1]. Example of post-processing experimental data for soliton enumeration. The top image is the destructive absorption image taken at the end of propagation. The middle image is the noise-reduced absorption image. Noise reduction is performed by DCT thresholding using $16 \times 16$ pixel blocks. The bottom image shows the connected components of the binarized middle image.

## II. INTERPLAY BETWEEN RESHAPING AND MODULATIONAL INSTABILITY

Here we analyze in more detail the role played by condensate reshaping (linear and nonlinear) as well as its mutual interplay with MI.

We show the existence of two distinct regimes that are dominated by reshaping and MI, respectively. We finally discuss an intermediate regime where reshaping and MI are both important to the condensate dynamics.

Numerical simulations discussed below are related to the solution of the 1D NPSE [Eq. (1) in the main text], where the system parameters are those of the experiment: $N = 3 \times 10^4$ is the number of $^{85}$Rb bosons in the condensate; $m \approx 85\,u$ is the corresponding atomic mass; $\omega_\perp = 2\pi \times 70$ Hz is the trapping frequency in the transverse direction. We set the s-wave scattering length $a_s = -a_0$ ($a_0$ is the Bohr radius). The initial axial function $f(z, t = 0)$ is described by a supergaussian of order 2: $f(z, t = 0) = ne^{-z^4/L_z^4}$, $n$ being a normalization factor such that the integral $\int |f(z, 0)|^2 \, dz = 1$. We analyze the axial spectrum of the condensate, that is, the intensity of the Fourier transform in $z$ of $f(z, t)$. Moreover, we vary the axial width $L_z$ of the condensate in order to enter the different aforementioned regimes.

### A. MI REGIME

When we fix $L_z = 1500\mu$m the condensate undergoes a strong MI effect that determines its dynamics. In this case, reshaping induced by diffraction is negligible because its characteristic timescale $T_\mathrm{D}$ is much longer than that related to nonlinear effects, $T_\mathrm{NL}$. Moreover, SPM is also negligible because the width $\Delta k$ of the initial axial spectrum is much smaller than the MI peak frequency $\hat{k}$ (see Fig. [S2]b). In order to demonstrate that the condensate dynamics are unaffected by diffraction and SPM, we simply run the simulation without seeding noise. Results in Figs. [S2]a,b clearly show that at $t = 7$s the shape of the density distribution $|f|^2$ and the corresponding spectrum are practically unchanged, confirming that the presence of diffraction and SPM do not play any relevant role. On the contrary, when a seeding noise is employed in the simulation, the condensate axial shape is strongly modified by MI. Figs. [S2]c,e show that running two simulations with different seeding noise yields a different pattern of separated components. Therefore, the random position, shape, and number of components is actually a clear signature of MI in the spatial domain. Another interesting MI-feature comes from the spectra in Figs. [S2]d,f; we clearly observe the raising of MI-bands

that are in full agreement with the theoretical MI-bands calculated from Eq. (3) of the main text. To conclude: both in the spatial and in the spectral domain we have a strong signature of an MI regime.

### B. RESHAPING REGIME

If we strongly shrink the initial condensate in the axial direction, then the perturbed plane wave approach typically employed in the description of MI cannot capture the true condensate dynamics, which is actually dominated by the reshaping due to both diffraction and SPM. Figure [S3] displays (at $t = 0.2$s) the input and output density distributions of the condensate and their corresponding spectra when $L_z = 5\mu$m. Panels a,b refer to the instance in which no seeding noise is applied, whereas panels c,d to the instance where a seeding noise is applied whose statistics is the same as the seeding noise used to produce Figs. [S2]c-f. As shown in Fig. [S3]d, in this case the initial spectrum width $\Delta k$ is large enough to completely overlap the MI-band. Therefore, the SPM causes a strong spectral broadening which is totally independent of the underlying seeding noise. Contrary to the case of Fig. [S2], here panels b,d clearly show that the output spectrum is practically unaffected by seeding noise and the same applies to the output density distributions (panels a,c). The dynamics are then fully deterministic and, at a fixed time $t$, we observe almost the same density distribution whatever the seeding noise is.

It is worth examining the full spatio-temporal evolution of the density distribution, which is shown in Fig. [S4]. We see that the condensate alternately experiences a compression and broadening in the axial direction, which is due to the mutual interplay between SPM and diffraction. The first induces a strong compression, that is the spatial counterpart of the spectral broadening, whereas the second counterbalances the SPM and tends to widen the condensate once it has been compressed. As a result, the full dynamics is almost periodic and resembles the dynamics experienced by short optical pulses in Kerr-media. On the other hand, several different spatio-temporal evolutions can be observed depending on the particular shape of the input condensate as well as on the linear and nonlinear coefficients of the system ($c_{1,2,3,4}$ in Eq. (1) of the main text).

### C. INTERMEDIATE REGIME

From the above considerations, we may expect that an intermediate regime exists where neither MI nor reshaping are dominant. In order to explore such a regime, we fix $t = 0.2$s and $L_z = 45\mu$m, which is similar to the input axial width in our experiments (see Fig. 2 of the main text). Following the same procedure employed for the MI regime and the reshaping regime, we first run the simulation in the absence of seeding noise. We see in Figs. [S5]a,b that if the noise is absent then the dynamics is driven by a strong reshaping. On the other hand, when noise is introduced, MI also plays a non-negligible role and gives rise to the formation of components, similarly to the case of a pure MI regime (see Figs. [S5]c-f). Most importantly, the output density distribution exhibits the typical MI-signature which is represented by a random position and shape of the components. However, in this case a partial correlation among components (i.e. ‘humps’) in different runs is present (see humps-A,B in panels c and e), which is due to the interplaying deterministic reshaping.

Note also that the creation of well-defined and separated components occurs on a timescale $\lesssim$ 90ms, in agreement with experimental results (see Fig. 2 of the main text).

## III. STATISTICAL COMPARISON OF SPATIAL COMPONENT DISTRIBUTIONS

In Figs. 4 and 5 of the main text, we compare the number of spatial components experimentally measured after breakup to 1D NPSE simulations (only in the regime $a_s \leq -1.7a_0$ where a negligible thermal population was observed and mean-field theory is valid). In order to determine whether the predictions of this theoretical model are in good agreement with the experimental data, we apply the independent samples $t$-test for unequal variances (i.e. Welch's $t$-test). This allows us to assess the difference between the theoretically-predicted and experimentally-measured distributions for each quenched scattering length. We did *not* assume equal variance between the two distributions, as we do not have a detailed *a priori* understanding of the technical noise sources within the experiment that lead to the stochastic variation in component breakup.

The results of our analysis are shown in Table [S1]. Since all $t$-tests returned $p > 0.05$, we conclude that the distribution of components in the experiment did not significantly differ from the distribution of components predicted by the NPSE.

| Scattering length ($a_0$) | $t$ statistic | df | $p$ value |
|---|---|---|---|
| -0.200 | .838 | 9.318 | .423 |
| -0.517 | .683 | 9.344 | .511 |
| -0.750 | -1.346 | 71.670 | .183 |
| -0.832 | -.560 | 9.226 | .589 |
| -1.148 | -1.278 | 9.376 | .232 |
| -1.463 | -2.241 | 9.178 | .051 |

TABLE [S1]. Results of $t$-tests for each quenched scattering length. For each test, we report the $t$-statistic, the degrees of freedom (df), and $p$ value.

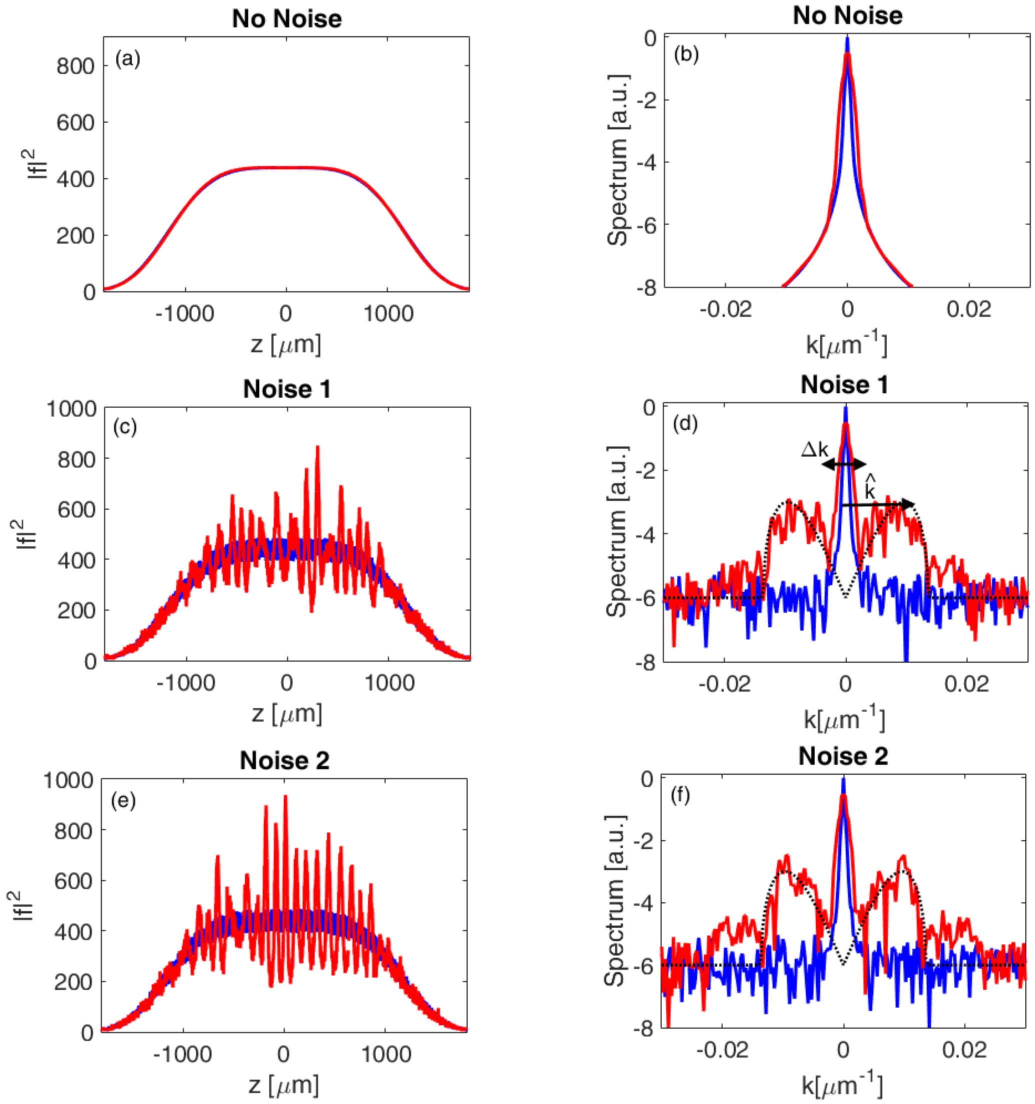


FIG. [S2]. Input (blue) and output (red) density functions (panels a,c,e) and corresponding spectra (panels b,d,f) when $L_z = 1500\mu$m and $t = 7$s. Panels a,b: no seeding noise. Panels c,d: seeding with noise 1. Panels e,f: seeding with noise 2. Noise 1 and 2 are different but possess the same statistics. Dotted black line in panels d and f represent the theoretical MI-band. Spectra are in dB.

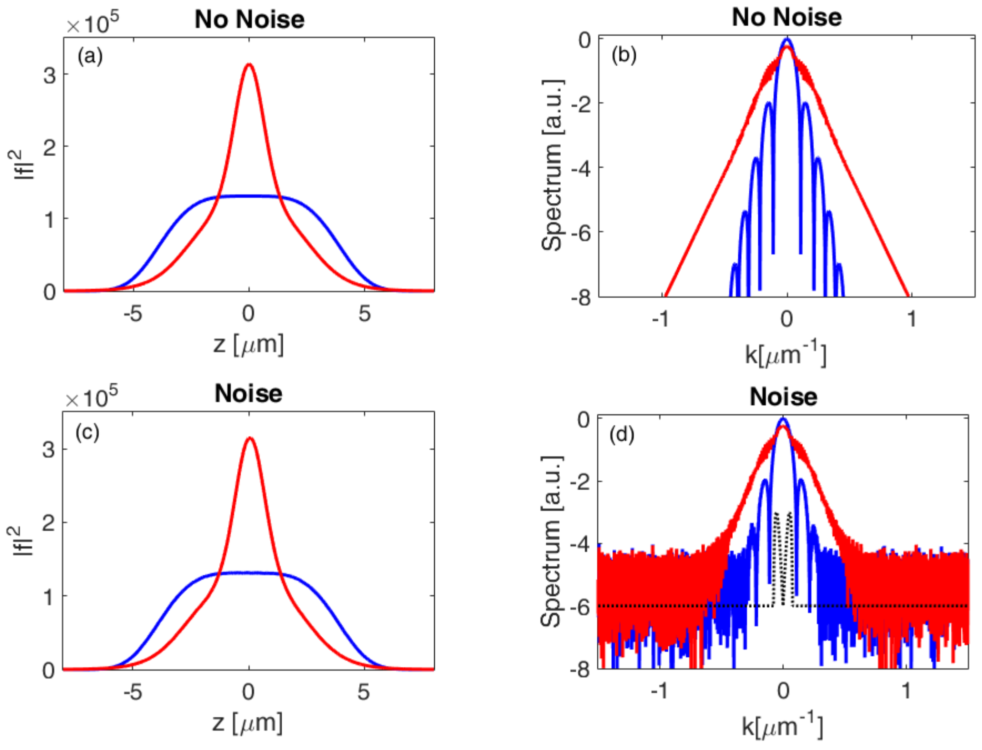


FIG. [S3]. Same as Fig.![S2], but for $L_z = 5\mu$m and $t = 0.2$s. Panels a,b: no seeding noise. Panels c,d: seeding with noise.

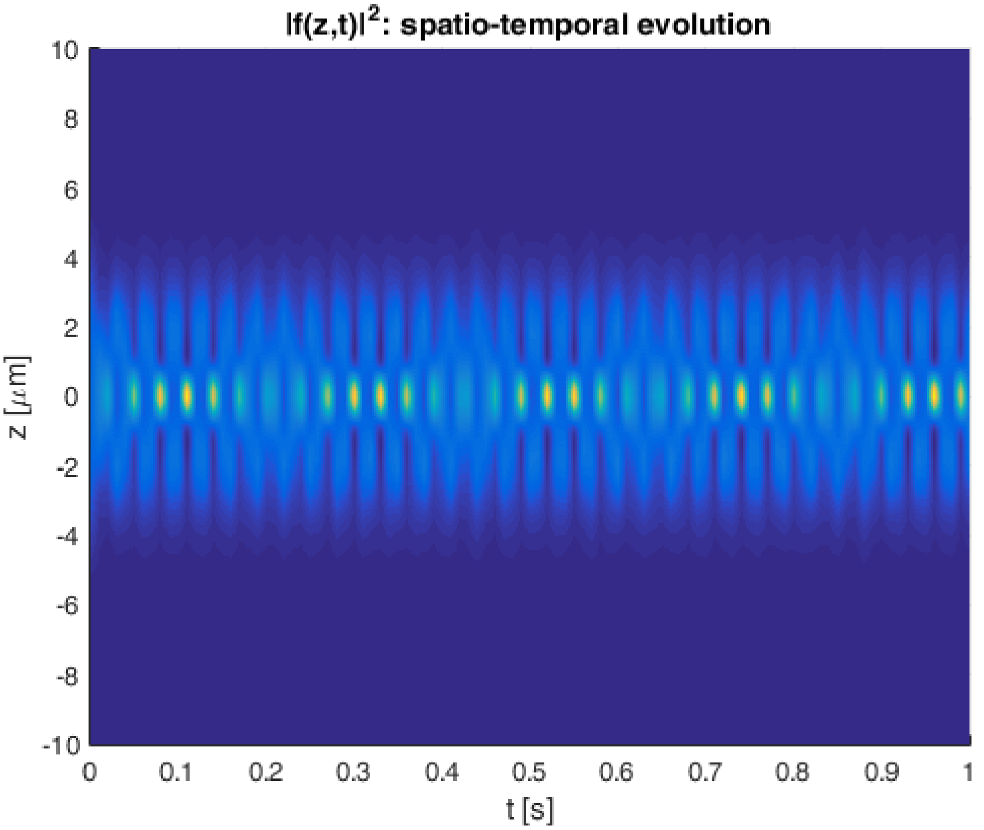


FIG. [S4]. Spatio-temporal evolution of the density distribution $|f|^2$ for $L_z = 5\mu$m and $t = 0.2$s. In this instance the evolution, which is dominated by reshaping, is quasi-periodic.

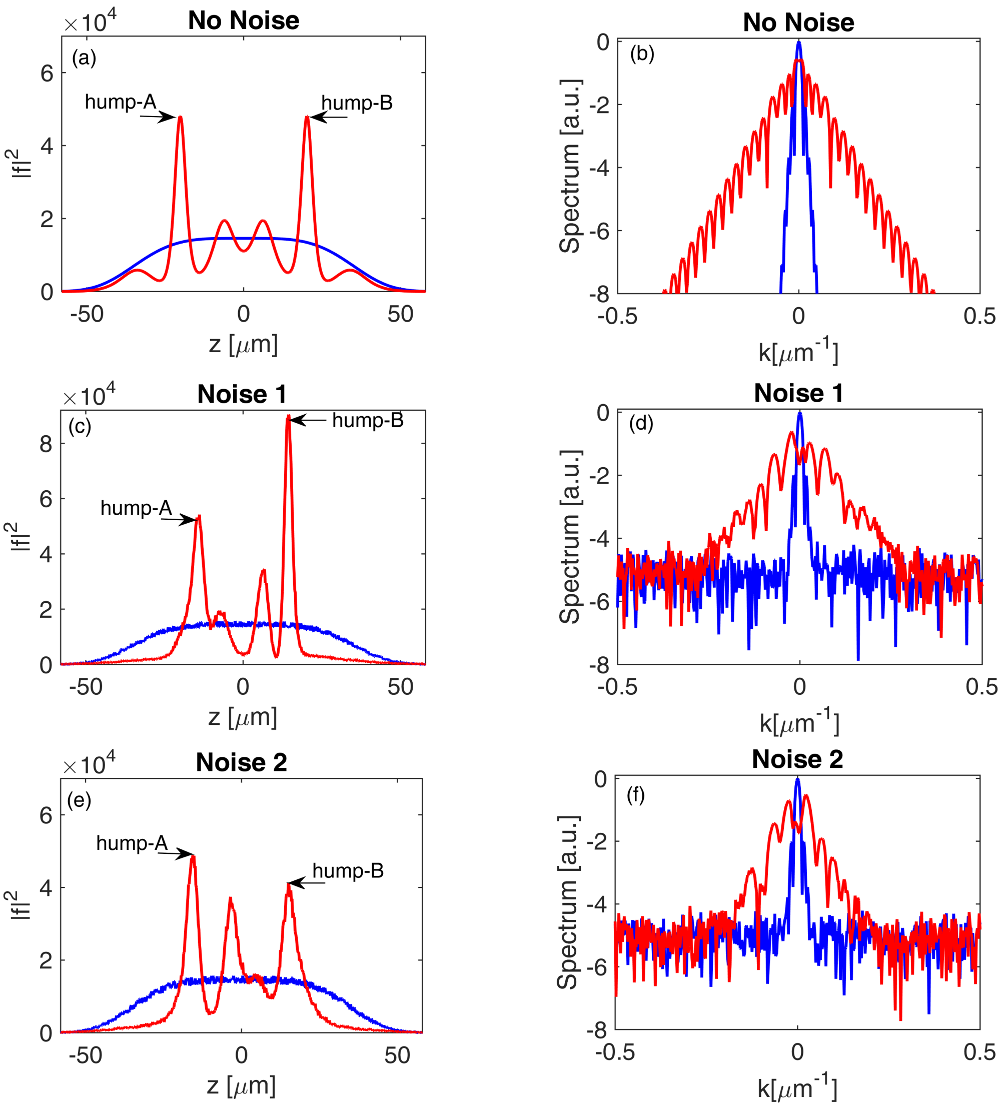


FIG. [S5]. Same as Fig. [S2], but for $L_z = 45\mu$m and $t = 0.2$s. Lateral humps (i.e. components) in the output density function are highlighted in panels a,c,e, showing the partial correlation between their position in the absence and presence of noise, respectively.
